# Supplementary material for: LLM-PQA: LLM-enhanced Prediction Query Answering
Source: arXiv:2409.01140 source file (2024-09-02)
Supplement: Supplementary file 1 [file appendix.tex]

\newpage
\section{Appendix}

\subsection{UI: determine user intent based on input message}

\begin{verbatim}
    prompt = f"""
    Based on the user's input, categorize and direct the action as follows:

    - If the input is a direct query like:
        "predict insurance charge for a 19 year old female, non-smoker, living in northeast with a BMI of 27.9 and no children"
        "predict real estate price with transaction date 2012.917, house age 32, distance to the nearest MRT station 84.87882, number of convenience stores 10, latitude 24.98298, longitude 121.54024"
        "please recommend playlist based on user id 4407"
       Respond as "query".

    - If the input is an affirmative response like:
        "y"
        "yes"
        "I want to use matched model and dataset"
      Respond as "confirm".

    - If the input suggests a desire for a new model, like:
        "new"
        "I want to use new model"
        "Can I select another model?"
        "I want to train a new model"
      Respond with "change". 
      
    - If the input specifies a choice for a new model like:
        "ClassificationModel"
        "I want to use model RegressionModel"
      Respond with "selection".

    - For input requesting help or instructions like:
        "how to use this system"
        "help"
        "user guide"
      Respond with "guide"

    - For any other type of input
      Respond with "chat"

    User input: "{prompt}"
    """
\end{verbatim}
\subsection{NL to SQL: determine whether NL to SQL is necessary}
\begin{verbatim}


    prompt = f"""
    The user query is: "{user_query}"

    Determine if this query requires data preprocessing. 
    The query will contain two parts: 
    - one part with requirements for data preprocessing 
    (e.g., "only consider house age less than 30", "from the 
    past six months"), 
    - and another part with information for machine learning tasks 
    (e.g., "predict real estate price with transaction date 
    2012.917, house age 32, distance to the nearest MRT 
    station 84.87882, number of convenience stores 10, 
    latitude 24.98298, longitude 121.54024", 
    "please recommend product id based on customer id 7172").

    If the query includes any data preprocessing requirements, 
    respond with a simple "yes".
    If the query only contains machine learning tasks and does 
    not require any data preprocessing, respond with a simple "no".

    Examples:
    1. Query: "only consider female data from the dataset, 
    predict insurance charge for a 19 year old female, 
    non-smoker, living in northeast with a BMI of 27.9 and no children"
       Response: "yes"
    2. Query: "predict insurance charge for a 19 year old female, 
    non-smoker, living in northeast with a BMI of 27.9 and no children"
       Response: "no"

    Respond only with "yes" or "no".
    """

\end{verbatim}
    
\subsection{NL to SQL: generate and execute code}
\begin{verbatim}

    prompt = f"""
    User Query: {user_query}
    Dataset Example: {sample_data}
    Dataset File Path: {selected_file_path}

    Please generate a Python code snippet to read the given CSV file and preprocess the data based on the user's query. The query will contain two parts: one part with requirements for data preprocessing (e.g., "only consider house age less than 30", "from the past six months"), and another part with information for machine learning tasks (e.g., "predict real estate price with transaction date 2012.917, house age 32, distance to the nearest MRT station 84.87882, number of convenience stores 10, latitude 24.98298, longitude 121.54024", "please recommend product id based on customer id 7172").

    Ignore the machine learning task information and only handle the data preprocessing requirements.

    Here are some examples for clarification:
    1. If the query is "only consider female data from the dataset, predict insurance charge for a 19 year old female, non-smoker, living in northeast with a BMI of 27.9 and no children", only filter the dataset to include female data, as shown below:
    
    ```python
    import pandas as pd

    # Read the CSV file
    data = pd.read_csv('D:/Program Files/Code repositories/RAG/RAG/rag_search/database_files/insurance.csv')

    # Keep only female data
    processed_data = data[data['sex'] == 'female']
    ```

    2. If the query is "only consider house age less than 30, predict real estate price with transaction date 2012.917,  house age 32, distance to the nearest MRT station 84.87882, number of convenience stores 10, latitude 24.98298, longitude 121.54024", only filter the dataset to include houses less than 30 years old, as shown below:

    ```python
    import pandas as pd

    # Read the CSV file
    data = pd.read_csv('D:/Program Files/Code repositories/RAG/RAG/rag_search/database_files/Real_estate.csv')

    # Filter houses with age less than 30
    processed_data = data[(data['X2 house age'] < 30)
    ```
    Ensure that the file paths in the generated code use double backslashes (\\\\) for Windows compatibility, and store the preprocessed data in a variable named 'processed_data'.
    """

\end{verbatim}
\subsection{model: select feature columns}
\subsubsection{linear regression}
\begin{verbatim}
        prompt = f"""
            Given the columns {self.data.columns.tolist()} in a 
            dataset and a user's query related to regression 
        analysis, the user's query is: '{self.query}'. 
            The task involves predicting a numerical outcome 
        based on various input features. 
            
            Based on the user's query and the available columns, 
            please suggest the most appropriate column names for: 
            1. Input variables: columns that will serve as input 
            features for predicting the outcome. 
            2. Output variable: the single column that represents the 
            target outcome to predict. 
            Please suggest all relevant columns as a single list in 
            the order they should be used for modeling, with the column
            representing the target outcome last, all separated 
        by a comma.
            For example, for a task to predict insurance charges based
            on a person's details, if the dataset columns are 
            ['age', 'bmi', 'children', 'charges', 'sex_female', 
            'sex_male', 'smoker_no', 'smoker_yes', 'region_northeast', 
            'region_northwest', 'region_southeast', 'region_southwest'],
            you should respond with: 'age', 'bmi', 'children', 
            'sex_female', 'sex_male', 'smoker_no', 'smoker_yes', 
            'region_northeast', 'region_northwest', 'region_southeast', 
            'region_southwest', 'charges'.
            please do not reponse like:" ["Input variables: 'age'", 
            " 'bmi'", " 'children'", " 'sex_female'", " 'smoker_no'", 
            " 'region_northeast'  \nOutput variable: 'charges'"]", 
            only reply with variables names like the example given 
            above.
            """
  
\end{verbatim}     
\subsubsection{recommendation task neural network}
\begin{verbatim}
        prompt = (
            f"Given the columns {self.data.columns.tolist()} in a 
            dataset and a user has made a request related to a binary 
            classification recommendation system."
            f"The user's request is: '{query}'. In a binary classification recommendation system, user IDs are typically linked 
            with item IDs to predict user preferences, such as music artist recommendations or playlist suggestions based on user interactions."
            f"Based on the user's request, please suggest the most appropriate column names for:"
            f"1. User IDs: typically a column identifying unique users."
            f"2. Item IDs: a column identifying items that can be recommended such as artists, tracks, or playlists."
            f"Please provide the column names for User IDs and Item IDs, separated by a comma without any spaces or quotation marks. For example, if the request is to recommend more musicians based on user names, respond with user_id,artistname. If the request is to recommend playlists based on user names, respond with user_id,playlistname."
        )

\end{verbatim}

\subsection{extract_features_with_llm}
\begin{verbatim}
        prompt = (
            f"Given the user query: '{query}', extract the following features: {', '.join(features)}. Provide the extracted values in the order they should be used for modeling. "
            f"For example, for a query 'predict insurance charge for a 19 year old female, non-smoker, living in northeast with a BMI of 27.9 and no children', and features are ['sex_female', 'sex_male', 'smoker_no', 'smoker_yes', 'region_northeast', 'region_northwest', 'region_southeast', 'region_southwest', 'age', 'bmi', 'children'], you should reply with '1, 0, 0, 1, 1, 0, 0, 0, 19, 27.9, 0'."
        )
\end{verbatim}

\subsection{recommendation task neural network extract user id}
\begin{verbatim}

    prompt = f"""
        Given the user's query: '{query}', please identify and extract the unique user ID. 
        The user ID might be a numeric ID, a hexadecimal string, or any form of unique identifier embedded in the query.
        Please return only the numeric user ID. For example, if the query content is "please recommend playlist based on use id 4407", return "4407".
        """

\end{verbatim}
\subsection{generate model name}
\subsubsection{linear regression}
\begin{verbatim}

    prompt = f"""
        Given the dataset with columns {self.data.columns.tolist()} and using input features {self.features} with target {self.target}, this model will perform linear regression analysis based on the user's query: '{self.query}'.
        Please generate a concise and descriptive model name that includes the term 'linear_regression' and clearly reflects its purpose. The model name should:
        1. Not exceed 30 characters in length.
        2. Include only the model name, without spaces or special characters, and be suitable for filenames.
        For example, a suitable model name for a task predicting house prices based on location and size could be 'house_price_linear_regression'.
        Please only reply with the model name.
        """

\end{verbatim}
\subsubsection{recommendation task neural network}
\begin{verbatim}

    prompt = f"""
        Given the dataset with columns {self.data.columns.tolist()} and a recommendation system using the columns '{self.user_col}' for user IDs and '{self.item_col}' for item IDs, alongside the user's request: '{query}':
        Generate a unique and descriptive model name that reflects the purpose and functionality of the model. This name should be suitable for identifying the model's files and its profile.
        Please provide the model name in a concise format, suitable for filenames, without spaces or special characters.
        For example, if you want to name a model as useridplaylistrecommender, do not answer "modelname: useridplaylistrecommender", only answer "useridplaylistrecommender"
        """

\end{verbatim}
\subsection{generate model profile}
\subsubsection{linear regression}
\begin{verbatim}

    prompt = f"""
        Create a detailed model profile for '{model_name}' based on the following specifications:

        - Model Name: {model_name}

        - Dataset Name: {self.dataset_name}

        - Model Overview: A linear regression model designed to predict outcomes based on numerical inputs. This model, utilizes input features {self.features} to predict the target {self.target} as influenced by the user's query: '{self.query}'.

        -Intended Use: This model is intended for use in sectors like real estate, finance, or any field where predicting continuous outcomes is valuable. It helps in making informed decisions by providing estimates based on historical data inputs.

        - Technical Details:
            Algorithm Type: Linear Regression
            Input Features: {self.features}
            Output: Predicted value of {self.target}

        - Model Performance:
            Mean Squared Error (MSE): {self.mse},
            R² Score: {self.r2}

        - Limitations:
            Linear regression assumes a linear relationship between input variables and the target. It may perform poorly if this assumption is violated or if the data contains high multicollinearity or outliers.

        For example, for a model profile name "insurancecharge_linear_regression" with dataset name "insurance", you should generate model profile like:
        Model Name: insurancecharge_linear_regression

        Dataset Name: insurance

        Model Overview:
        The insurancecharge_linear_regression model is trained on the insurance dataset to predict insurance charges based on a human's medical information. It utilizes input features such as age, BMI, number of children, gender, smoking habit, and region, to estimate the charges a person might incur for insurance coverage.

        Intended Use:
        This model is designed for predicting insurance charges based 
        on individual medical information. It can be utilized by 
        insurance companies, healthcare providers, or individuals 
        seeking estimates for insurance premiums. It enables 
        informed decision-making by providing accurate predictions 
        based on the input variables.

        Technical Details:
        - Algorithm Type: Linear Regression
        - Input Features: ['age', 'bmi', 'children', 'sex_female', 'sex_male', 'smoker_no', 'smoker_yes', 'region_northeast', 'region_northwest', 'region_southeast', 'region_southwest']
        - Output: Predicted value of insurance charges

        Model Performance:
        - Mean Squared Error (MSE): 33497825.55368333
        - R² Score: 0.7615425718903163

        Limitations:
        - Linear regression assumption: The model assumes a linear relationship between input variables and insurance charges. If this assumption is violated, the model's performance may be affected.
        - Multicollinearity and outliers: High multicollinearity among input features or presence of outliers in the data can impact the model's accuracy and reliability in predicting insurance charges.
        """

\end{verbatim}
\subsubsection{recommendation task neural network}
\begin{verbatim}

    prompt = f"""
        Create a detailed model profile for '{model_name}' based on the following specifications:

        Model Name:
        {model_name}

        Model Overview:
        A binary classification recommendation system designed to suggest items (like artists or products) based on user interactions. The system uses columns '{self.user_col}' and '{self.item_col}' from a dataset to train a model aimed at fulfilling the user's specific request: '{query}'.

        Intended Use:
        This model is intended to be used in environments where personalization and user preference prediction are critical, for example in e-commerce or entertainment platforms, to enhance user experience by accurately predicting and recommending items.

        Technical Details:
        Algorithm Type: Mixed Collaborative Filtering with Neural Networks
        Input Features: User IDs and Item IDs from columns '{self.user_col}' and '{self.item_col}'
        Output: Probability scores indicating user preference

        Model Performance:
        - Accuracy: {self.performance_metrics['accuracy']}
        - Precision: {self.performance_metrics['precision']}
        - Recall: {self.performance_metrics['recall']}

        Limitations:
        Performance may degrade with sparse user-item interactions or limited diversity in the training data set.

        Please format the profile to be clear, professional, and detailed.
        """

\end{verbatim}

\subsection{generate dataset profile}
\subsubsection{linear regression}
\begin{verbatim}

    prompt = f"""
        Create a detailed dataset profile for '{self.dataset_name}' based on the following specifications:

        - Dataset Name: {self.dataset_name}

        - Overview: This dataset contains data structured in several columns: {column_names}. Below is a sample of the data to provide insight into the typical content and structure of the dataset:

            {sample_data}

        - Usage: This dataset is primarily used for building predictive models in the {dataset_name.split('_')[0]} domain. 

        For example, is the dataset name is Real_estate, you should generate a dataset profile like:

        Dataset Name: Real_estate

        Overview: This dataset contains comprehensive information related to real estate transactions, structured across several columns: ['No', 'X1 transaction date', 'X2 house age', 'X3 distance to the nearest MRT station', 'X4 number of convenience stores', 'X5 latitude', 'X6 longitude', 'Y house price of unit area']. Below is a sample of the data to provide insight into the typical content and structure of the dataset:
        No, X1 transaction date, X2 house age, X3 distance to the nearest MRT station, X4 number of convenience stores, X5 latitude, X6 longitude, Y house price of unit area 1, 2012.917, 32, 84.87882, 10, 24.98298, 121.54024, 37.9 2, 2012.917, 19.5, 306.5947, 9, 24.98034, 121.53951, 42.2 3, 2013.583, 13.3, 561.9845, 5, 24.98746, 121.54391, 47.3 4, 2013.500, 13.3, 561.9845, 5, 24.98746, 121.54391, 54.8 5, 2012.833, 5, 390.5684, 5, 24.97937, 121.54245, 43.1 6, 2012.667, 7.1, 2175.03, 3, 24.96305, 121.51254, 32.1 7, 2012.667, 34.5, 623.4731, 7, 24.97933, 121.53642, 40.3 8, 2013.417, 20.3, 287.6025, 6, 24.98042, 121.54228, 46.7 9, 2013.500, 31.7, 5512.038, 1, 24.95095, 121.48458, 18.8 10, 2013.417, 17.9, 1783.18, 3, 24.96731, 121.51486, 22.1

        Usage: The Real_estate.csv dataset is extensively employed in predictive analytics projects focused on real estate market trends. It's particularly useful for developing machine learning models to predict property prices based on various attributes such as age, proximity to amenities, and geographical coordinates. This dataset supports a wide range of real estate market analyses, from understanding price determinants to forecasting future price movements in different regions.
        """

\end{verbatim}
\subsubsection{recommendation task neural network}
\begin{verbatim}

        prompt = f"""
        Create a detailed dataset profile based on the following specifications:

        Dataset Name: {dataset_name}

        Overview:
        This dataset contains data structured in several columns: {column_names}. Below is a sample of the data to provide insight into the typical content and structure of the dataset:

        {sample_data}

        Usage:
        This dataset is primarily used for building recommendation models in the {dataset_name.split('_')[0]} domain. 

        Please format the profile to be clear, professional, and detailed.
        """
\end{verbatim}

\section{System architecture}

The system architecture of \ziyu{DEMONAME} is designed to seamlessly integrate vector search capabilities with large language models (LLMs) and machine learning inference. The architecture is built to efficiently handle diverse and complex queries by dynamically selecting the most appropriate models and datasets. The main components and their interactions are outlined below.

\paragraph{Main Components}

\begin{itemize}
    \item \textbf{User Interface (UI)}:
    \begin{itemize}
        \item \textit{Chatbot Interface}: This component captures user inputs and displays system responses, facilitating an intuitive and interactive query process.
        \item \textit{Chat History Management}: Stores and manages the chat history for each user session, ensuring continuity and context in user interactions.
    \end{itemize}
    
    \item \textbf{Query Processing Unit}:
    \begin{itemize}
        \item \textit{Intent Recognition}: Uses LLMs to interpret the user's query and identify the required actions.
        \item \textit{Vector Search Engine}: Utilizes MongoDB Atlas to perform vector searches, matching the user's query with the most relevant model and dataset profiles.
    \end{itemize}
    
    \item \textbf{Model and Data Management}:
    \begin{itemize}
        \item \textit{Model Zoo}: A collection of pre-trained machine learning models that can be dynamically selected based on the query requirements.
        \item \textit{Data Lake}: A storage repository that holds a vast amount of raw data in its native format until it is needed, supporting diverse data types and structures.
    \end{itemize}
    
    \item \textbf{Model and Data Alignment}:
    \begin{itemize}
        \item \textit{Alignment Verification}: Ensures the selected model and dataset are correctly aligned by comparing dataset names in their respective profiles.
    \end{itemize}
    
    \item \textbf{Data Preprocessing Module}:
    \begin{itemize}
        \item \textit{NL to SQL Conversion}: Uses LLMs to convert natural language preprocessing instructions into SQL or equivalent code.
        \item \textit{Execution Engine}: Executes the generated code to preprocess the data as specified by the user's query.
    \end{itemize}
    
    \item \textbf{Model Navigator}:
    \begin{itemize}
        \item \textit{Model Selector}: Guides the selection of the appropriate machine learning model based on the user's query and the available models.
        \item \textit{Handler Loader}: Loads the necessary handlers to prepare the selected model for query execution.
    \end{itemize}
    
    \item \textbf{Execution and Training Unit}:
    \begin{itemize}
        \item \textit{Query Execution}: Executes the query using the aligned model and dataset.
        \item \textit{Model Training}: Trains a new model using the selected dataset if the user opts for training a new model instead of using an existing one.
    \end{itemize}
    
    \item \textbf{Profile Generation and Database Management}:
    \begin{itemize}
        \item \textit{Profile Creator}: Generates detailed profiles for models and datasets, which include their specifications, performance metrics, and usage details.
        \item \textit{Database Uploader}: Uploads the generated profiles to MongoDB Atlas for future reference and use.
    \end{itemize}
    
    \item \textbf{Result Display}:
    \begin{itemize}
        \item \textit{Result Presenter}: Displays the final results of the query to the user, including relevant performance metrics and data insights.
    \end{itemize}
\end{itemize}

This architecture ensures that \ziyu{DEMONAME} is capable of handling a wide range of queries with high accuracy and contextual relevance, leveraging advanced technologies for data retrieval, preprocessing, and machine learning inference.

\subsection{Technologies and tools}

The \ziyu{DEMONAME} framework leverages several advanced technologies and tools to provide a robust and efficient system for handling diverse machine learning queries. Below, we describe the key technologies and tools used in the system:

\paragraph{MongoDB Atlas}

MongoDB Atlas is a fully-managed cloud database service that provides a flexible, scalable, and secure database solution. In our system, MongoDB Atlas is utilized primarily for its powerful vector search capabilities, which are essential for matching user queries with the most relevant model profiles and dataset profiles stored in the database. The integration of MongoDB Atlas in the Query Handling component allows the system to:

\begin{itemize}
    \item \textbf{Store Model and Dataset Profiles}: Profiles of various machine learning models and datasets are stored in MongoDB Atlas, allowing for efficient retrieval and management.
    \item \textbf{Perform Vector Search}: When a user inputs a query, the system converts the query into a vector representation. MongoDB Atlas then performs a vector search to find the model and dataset profiles that best match the query. This ensures that the most relevant resources are selected for processing the query.
    \item \textbf{Handle Large Volumes of Data}: MongoDB Atlas is capable of handling large volumes of data, which is crucial for storing extensive model and dataset profiles and ensuring quick access to them.
\end{itemize}

\paragraph{Natural Language to SQL (NL to SQL)}

The ability to process and understand natural language queries is a core feature of the \ziyu{DEMONAME} framework. Often, users may input queries that require specific data preprocessing steps before a model can be trained or used for prediction. For instance, a user might input: "only consider female data from the dataset, predict insurance charge for a 19 year old female, non-smoker, living in northeast with a BMI of 27.9 and no children". In such cases, the system needs to preprocess the dataset to include only the relevant subset of data (e.g., only female data).

To achieve this, the system employs Natural Language to SQL (NL to SQL) techniques, facilitated by Large Language Models (LLMs) like GPT-4 (ChatGPT API):

\begin{itemize}
    \item \textbf{Interpreting Natural Language Queries}: The system uses LLMs to parse and understand the natural language queries input by the user. This involves identifying the specific preprocessing instructions embedded in the query.
    \item \textbf{Generating SQL Code}: Once the preprocessing requirements are identified, the system uses LLMs to generate the appropriate SQL (or equivalent data manipulation code) to preprocess the dataset as specified. For example, for the query "only consider female data from the dataset", the system would generate an SQL command to filter the dataset to include only rows where the gender is female.
    \item \textbf{Executing the Code}: The generated code is then executed to preprocess the dataset. The preprocessed data is saved and used for subsequent model training or prediction tasks.
    \item \textbf{Ensuring Data Integrity and Efficiency}: By using NL to SQL, the system ensures that data preprocessing is done accurately and efficiently, allowing for seamless integration with the model training and prediction processes.
\end{itemize}

\paragraph{Ensuring Alignment of Models and Datasets}

Ensuring that the matched model and dataset are correctly aligned is critical for the accuracy and reliability of the \ziyu{DEMONAME} framework. Each model corresponds to a unique dataset, though a dataset can be used by multiple models. The system verifies the alignment of models and datasets through the following method:

\begin{itemize}
    \item \textbf{Profile Generation}: Each model and dataset has a corresponding profile stored in MongoDB Atlas. These profiles are generated using LLMs to ensure they follow a consistent and specific format.
    \item \textbf{Matching Process}: When a query is processed, the system performs a vector search to find the most relevant model and dataset profiles.
    \item \textbf{Alignment Check}: The system extracts the dataset name from the matched model profile and compares it with the dataset name extracted from the dataset profile. This comparison ensures that the dataset used to train the model matches the dataset intended for use with the query.
    \item \textbf{Consistency and Accuracy}: By enforcing this alignment check, the system ensures that the model's predictions are based on the correct data, maintaining the integrity and accuracy of the query results.
\end{itemize}

The profiles are generated using the ChatGPT API, where appropriate prompts are provided to create detailed and structured profiles. For example, when generating a profile for a linear regression model, the prompt includes specifications such as the model name, dataset name, an overview of the model, intended use, technical details, performance metrics, and limitations. This ensures that each profile contains all necessary information for effective matching and alignment verification.

These technologies and tools form the backbone of the \ziyu{DEMONAME} framework, enabling it to handle complex queries, perform efficient data retrieval and preprocessing, and deliver accurate and contextually relevant responses to users.

\subsection{Workflow example}

\begin{figure}
  \centering
  \includegraphics[width=\linewidth]{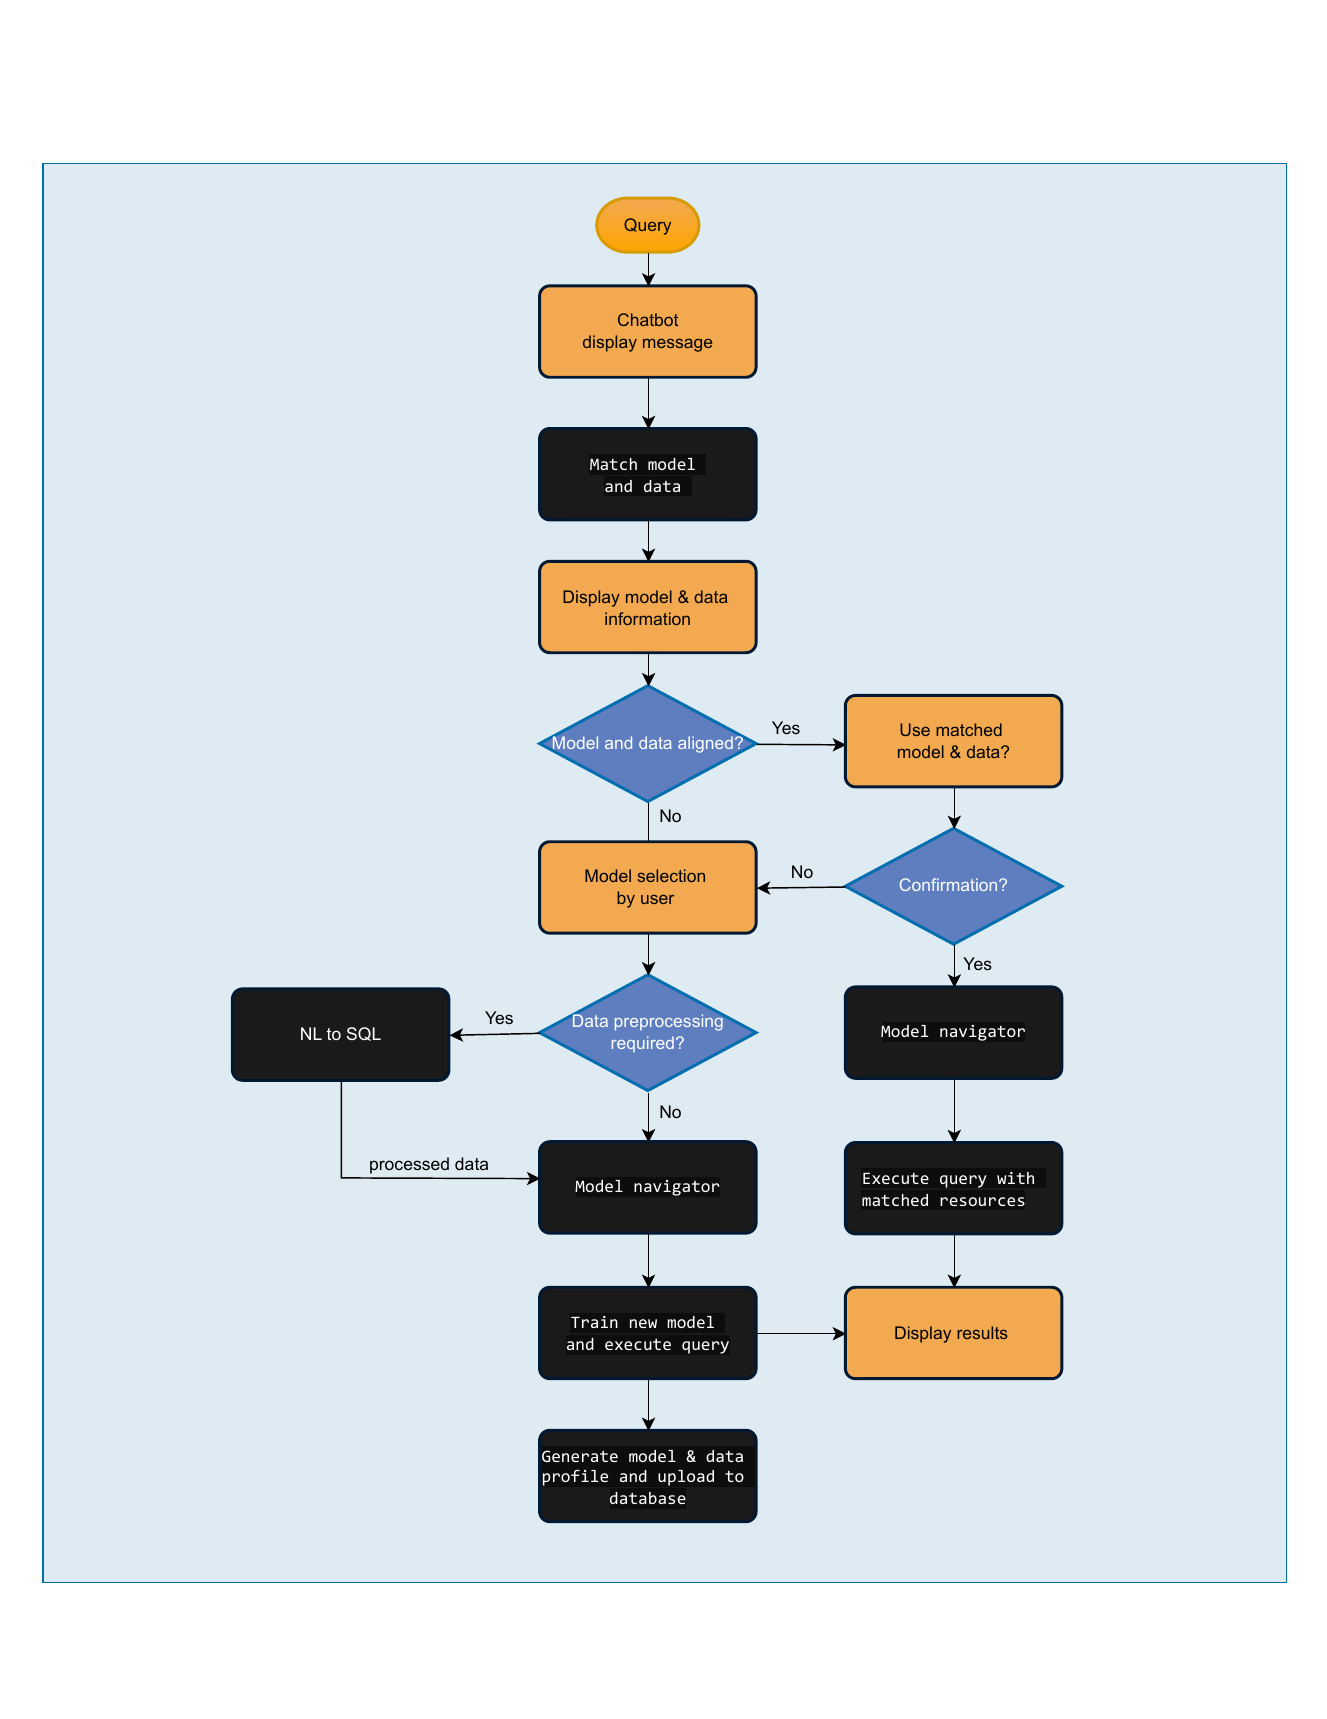}
  \caption{system flowchart}
  \label{fig:system flowchart}
\end{figure}

The workflow of \ziyu{DEMONAME} involves several steps to handle user queries, preprocess data if needed, and execute machine learning models to provide results. Here is a detailed example of the workflow:

\begin{enumerate}
    \item \textbf{User Input}: The user inputs a query through the chatbot interface.
    \item \textbf{Query Interpretation}: The system interprets the query using LLMs to determine the intent and required actions.
    \item \textbf{Vector Search}: The query is converted into a vector representation and matched with the most relevant model and dataset profiles using MongoDB Atlas.
    \item \textbf{Model and Data Display}: Information about the matched model and dataset is displayed to the user.
    \item \textbf{Alignment Check}: The system verifies if the matched model and dataset are correctly aligned.
    \item \textbf{Data Preprocessing}: If required, data preprocessing is performed using generated SQL or equivalent code.
    \item \textbf{Model Execution}: The system executes the query using the aligned model and dataset or trains a new model if requested.
    \item \textbf{Profile Generation}: Profiles for the model and dataset are generated and uploaded to MongoDB Atlas.
    \item \textbf{Result Display}: The final results, along with relevant information, are displayed to the user.
\end{enumerate}

This workflow ensures flexibility and robustness in handling a variety of user queries, enabling both the use of pre-trained models and the training of new models based on user inputs.

\subsection{Performance evaluation, limitation and future work}

\para{}

\para{}

\para{}
